# Supplementary material for: Deep Generation of Face Images from Sketches
Source: arXiv:2006.01047 source file (2020-06-05)
Supplement: Supplementary file 1 [file Appendix.tex]

%\section{Appendices}
